# Supplementary material for: Energy-adaptive Buffering for Efficient, Responsive, and Persistent Batteryless Systems
Source: arXiv:2401.08806 source file (2024-01-16)
Supplement: Supplementary file 1 [file appendix.tex]

\clearpage
\appendix
\section{Appendix}
\label{sec:appendix}
\input{Figures/traces_table.tex}
We evaluate \sys{} using five input power traces chosen to illustrate how environmental fluctuations affect energy harvesting systems using two of the most mature energy harvesting technologies: solar energy harvesting and RF radiation.
This appendix contains plots of the input power for each trace along with a short description of the environment and system behavior.
Table~\ref{table:traces} gives a short summary of each trace.

\subsection{RF Traces}
The RF traces are based on a commercial 915 MHz energy harvesting circuit~\cite{p2110b} using a dipole antenna which rectifies incoming energy from a 3W, vertically polarized transmitter~\cite{tx91501b}.
We use the integrated power measurement feature of the harvesting chip to determine received signal strength; the input power measured implicitly includes the efficiency of the RF-to-DC converter, but not the integrated boost converter.
We emulate the behavior of the boost converter (Section~\ref{sec:eh-replay}) based on the datasheet specifications.
All RF measurements are in an active office environment.

\begin{figure}[h]
 \centering
  \includegraphics[width=\columnwidth]{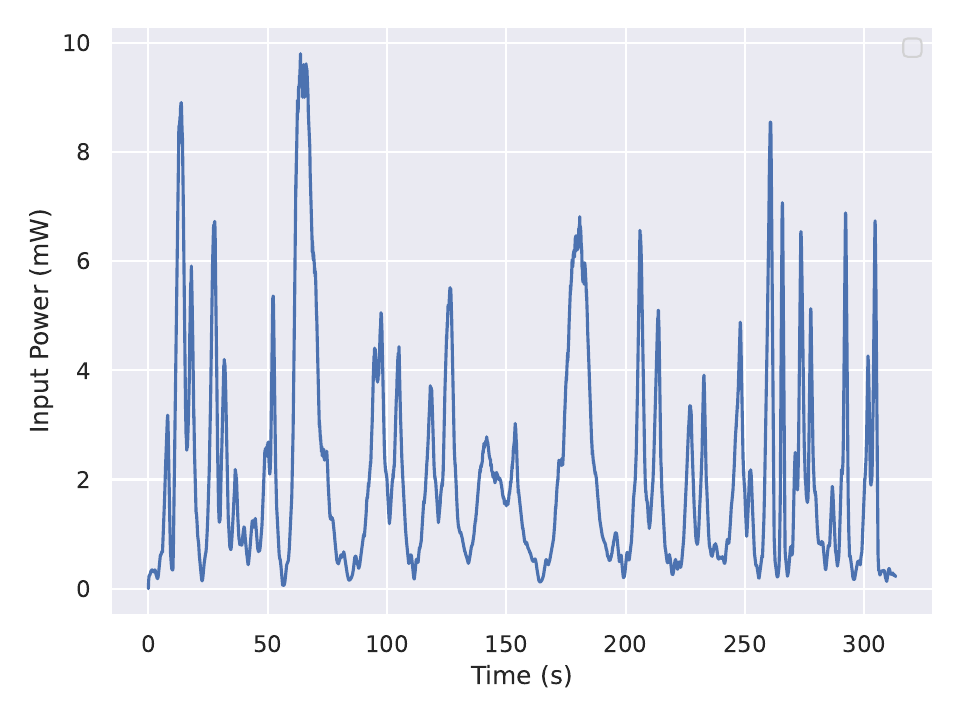}
  \caption{RF Cart: The harvester is on a small cart in the plane of the transmitter, repeatedly moving towards, away from, and around it.}
  \label{fig:dipole-cart}
\end{figure}
\begin{figure}[h]
 \centering
  \includegraphics[width=\columnwidth]{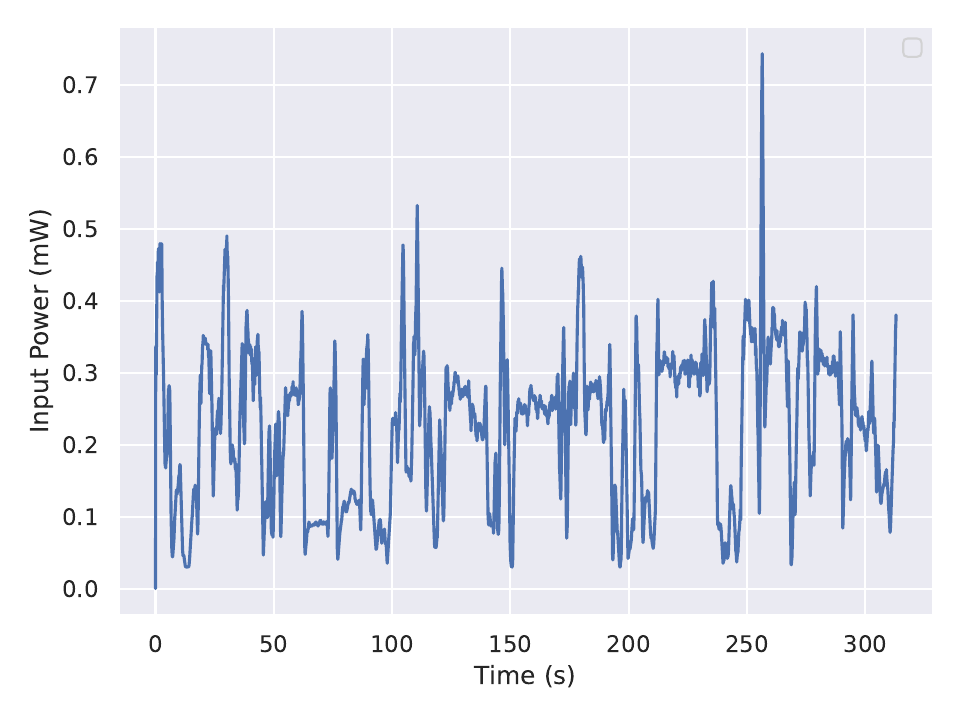}
  \caption{RF Obstruction: The harvester is stationary on a desk approximately 1 meter from and in the plane of the transmitter. Various obstructions (laptops, metal water bottles, etc.) are periodically moved between and around the transmitter and harvester.}
  \label{fig:dipole-obstructions}
\end{figure}
\begin{figure}[h]
 \centering
  \includegraphics[width=\columnwidth]{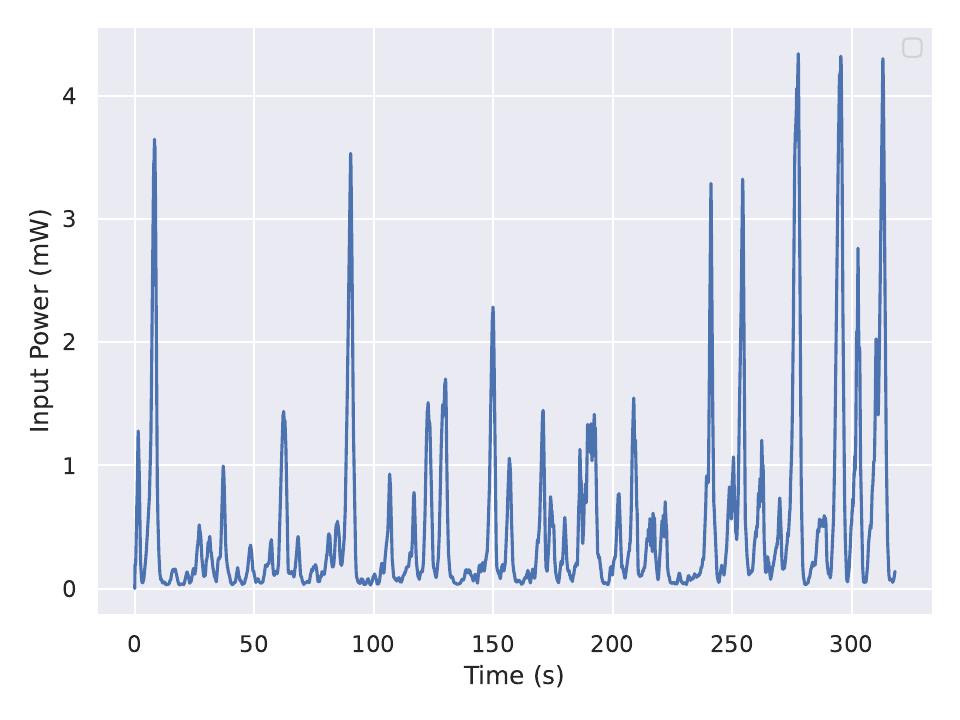}
  \caption{RF Mobile: The transmitter is mounted in the upper corner of a room, facing down towards the center of the room. The harvester is carried through, around, and out of the room.}
  \label{fig:dipole-mobile}
\end{figure}

\subsection{Solar Traces}
The solar traces are taken from the Enhants mobile irradiance dataset~\cite{enhants}.
We convert irradiance to usable input power emulating a 22\% efficient, 5 $cm^2$ solar panel~\cite{mini-solar-panel} connected to a commercial solar energy harvesting management circuit~\cite{bq25570}.

\begin{figure}[h]
 \centering
  \includegraphics[width=\columnwidth]{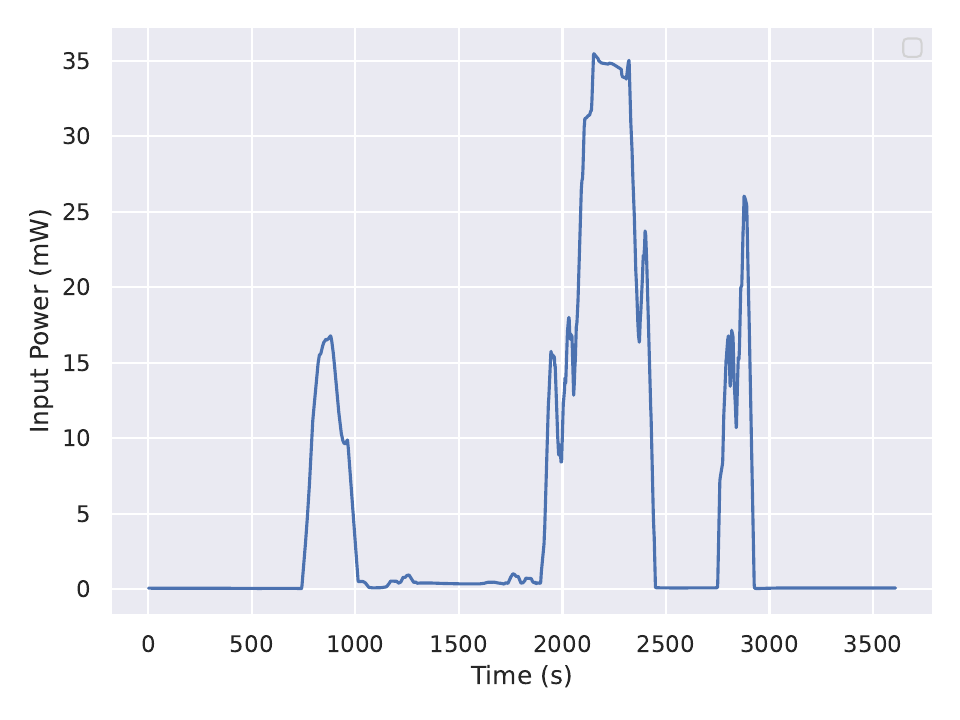}
  \caption{Solar Campus: Pedestrian walking around university campus (indoor and outdoor environments) carrying a sensor.}
  \label{fig:solar-campus}
\end{figure}
\begin{figure}[h]
 \centering
  \includegraphics[width=\columnwidth]{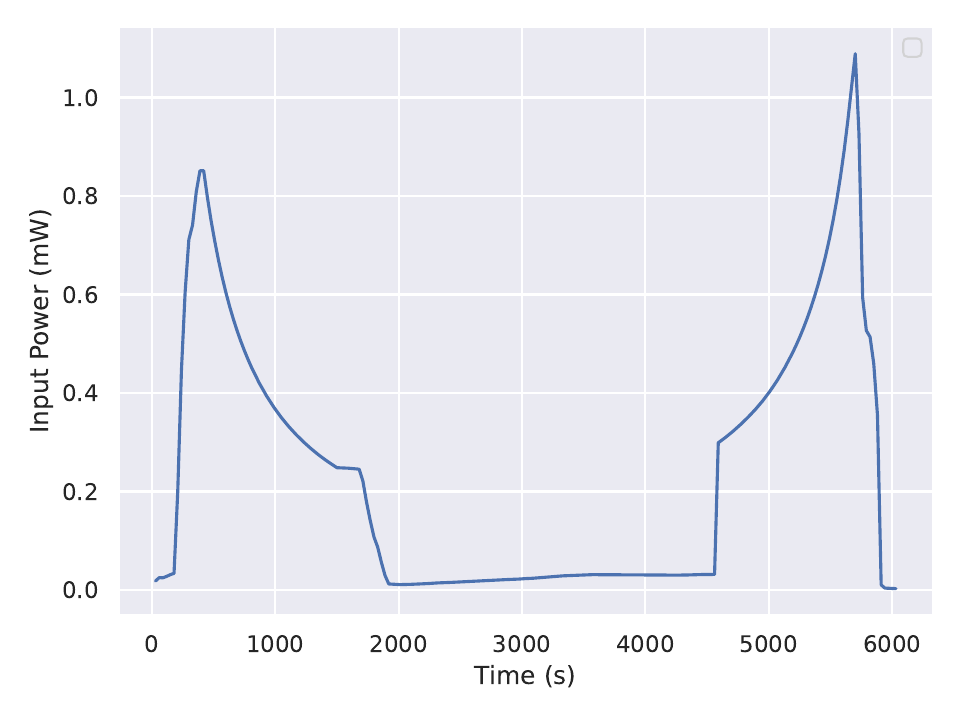}
  \caption{Solar Commute: Commuting on public transit, sensor attached to a backpack, measurements outdoors, indoors (office, subway, train).}
  \label{fig:solar-commute}
\end{figure}
